# Supplementary material for: Enhancing AUTOSAR-Based Firmware Over-the-Air Updates in the Automotive Industry with a Practical Implementation on a Steering System
Source: arXiv:2503.05839 source file (2025-03-18)
Supplement: Supplementary file 1 [file app0A.tex]

%
% file: localoperator.tex
% author: Victor Brena
% description: Briefly describes properties of the local operator.
%

\chapter{Appendix A}
\label{app:app01}

Begins an appendix

\
